# Supplementary material for: AltGeoViz: Facilitating Accessible Geovisualization
Source: arXiv:2406.13853 source file (2024-12-09)
Supplement: Supplementary file 1 [file Appendix.tex]

\section{Appendix}
\begin{table*}[]
\centering
\setlength{\extrarowheight}{5pt} 
\begin{tabular}{@{}cccllll@{}}
\toprule
\rowcolor[HTML]{FFFFFF} 
\textbf{PID} &
  \textbf{Gender} &
  \textbf{Age} &
  \textbf{Screen Reader} &
  \textbf{Vision-Loss Level} &
  \textbf{Education Level} &
  \textbf{\begin{tabular}[c]{@{}l@{}}Frequency of Interaction \\ with Online Maps\end{tabular}} \\ \midrule
\rowcolor[HTML]{F3F3F3} 
P1 & Male & 38 & JAWS & Lost vision gradually & Master’s degree   & 1-5  times a week       \\
\rowcolor[HTML]{FFFFFF} 
P2 & Male & 49 & JAWS & Lost vision gradually & Master’s degree   & 1-5  times a week       \\
\rowcolor[HTML]{F3F3F3} 
P3 &
  Male &
  60 &
  JAWS &
  \begin{tabular}[c]{@{}l@{}}Lost vision gradually, \\ Complete blindness\end{tabular} &
  Bachelor’s degree &
  Less than once per week \\
\rowcolor[HTML]{FFFFFF} 
P4 & Female & 54 & JAWS & Complete blindness    & Bachelor’s degree & 1-5  times a week       \\
\rowcolor[HTML]{F3F3F3} 
P5 & Female & 30 & NVDA & Blind since birth     & Master’s degree   & Less than once per week \\ \bottomrule
\end{tabular}%
\caption{Screen-reader participants, their gender, age, screen-reader used for the study, vision-loss level, education level and frequency of interaction with online maps.}
\label{tab:participant}
\end{table*}
